# Supplementary material for: An Exponential Lower Bound for Zadeh's pivot rule
Source: arXiv:1911.01074 source file (2020-10-30)
Supplement: Supplementary file 1 [file A1AppendixAssumptions.tex]

%!TEX root = ../Main.tex
\section{Abbreviations and Tables} \label{appendix: Explanations}

In this appendix we explain all abbreviations used in the proofs and properties of strategies introduced in the main part.
For all of these explanations let $\sigma\in\reach{\iota}$ be some strategy.
\Cref{table: Simple abbreviations} contains an overview of several boolean expressions.
These expressions are either true (i.e., equal to 1) or false (i.e., equal to~0).
They are used to have a compact representation of the state of the counter and to compare and link the configurations of different vertices.

\begin{table}[ht]
\footnotesize
\centering
\begin{tabular}{|l|l|} \hline
Symbol							&Encoded boolean expression			\\\hline\hline
$\sigmabar(b_i)$				&$\sigma(b_i)=g_i$					\\
$\sigmabar(s_{i,j})$			&$\sigma(s_{i,j})=h_{i,j}$			\\
$\sigmabar(g_i)$				&$\sigma(g_i)=F_{i,1}$				\\
$\sigmabar(d_{i,j,k})$			&$\sigma(d_{i,j,k})=F_{i,j}$		\\
$\sigmabar(e_{i,j,k})$			&$\sigma(e_{i,j,k})=b_2$			\\\hline
\end{tabular}
\hspace*{1em}
\begin{tabular}{|l|l|} \hline
Symbol					&Encoded boolean expression																\\\hline\hline
$\sigmabar(s_i)$		&$\sigmabar(s_{i,\sigmabar(g_i)})$														\\
$\sigmabar(d_{i,j})$	&$\sigmabar(d_{i,j,0})\wedge\sigmabar(d_{i,j,1})$										\\
$\sigmabar(d_i)$		&$\sigmabar(d_{i,\sigmabar(g_i)})$														\\
$\sigmabar(eg_{i,j})$	&$\bigvee_{k=0,1}\left [\nsigmabar(d_{i,j,k})\wedge\nsigmabar(e_{i,j,k})\right ]$		\\
$\sigmabar(eb_{i,j})$	&$\bigvee_{k=0,1}\left [\nsigmabar(d_{i,j,k})\wedge\sigmabar(e_{i,j,k})\right ]$		\\
$\sigmabar(eg_i)$		&$\sigmabar(eg_{i,\sigmabar(g_i)})$														\\
$\sigmabar(eb_i)$		&$\sigmabar (eb_{i,\sigmabar(g_i)})$													\\ \hline
\end{tabular}
\caption{Strategy notation and expressions.
For convenience, $\sigmabar(b_{n+1})\coloneqq 0$.} \label{table: Simple abbreviations}
\end{table}

We now define the properties used for defining the term 'Phase-$k$-strategy'.
As discussed in the main part, each property is a boolean expression that might depend on one or two parameters.
Further note that the properties also might depend on whether we consider PG or MDP context.
%For every strategy $\sigma$, each property is either true or false.

{\footnotesize
\begin{minipage}{0.54\textwidth}
\begin{align*}
\sigma(s_{i,\indbit_{i+1}^{\sigma}})=h_{i,\indbit_{i+1}^{\sigma}}\wedge\sigma(s_{i,1-\indbit_{i+1}^{\sigma}})=b_1 \label{property: Usv1} \tag{Usv1}\\[1pt]
\sigma(s_{i,j})=h_{i,j} \label{property: Usv2} \tag{Usv2}\\
\sigma(s_{i,\indbit_{i+1}^{\sigma}})\neq h_{i,\indbit_{i+1}^{\sigma}} \wedge \sigma(s_{i,1-\indbit_{i+1}^{\sigma}})\neq b_1 \label{property: Usv3} \tag{Usv3}\\
\nexists i\colon\sigma(b_{i-1})=g_{i-1}\wedge\sigmabar(b_i)\neq\sigmabar(g_{i-1}) \label{property: Rel1} \tag{Rel1}\\
\relbit{\sigma}=\nsb(\indbit^{\sigma}) \label{property: Rel2} \tag{Rel2} \\
i<\relbit{\sigma}\Rightarrow\neg\sigmabar(d_{i,0})\vee\neg\sigmabar(d_{i,1}) \label{property: Cc1} \tag{Cc1} \\
\sigmabar(d_{\nsb})\wedge\sigmabar(g_{\nsb})=(\bit+1)_{\nsb+1} \label{property: Cc2} \tag{Cc2}\\
\sigmabar(d_{i,j})\Rightarrow j\neq\indbit_{i+1}^{\sigma} \label{property: Cc3} \tag{Cc3} \\
\begin{aligned}
			\text{MDP-context: } \sigmabar(g_i)=1-\indbit^{\sigma}_{i+1}&\Rightarrow\sigmabar(d_{i,1-\indbit^{\sigma}_{i+1}})\\
			\text{PG-context: } \sigmabar(g_i)=1&\Rightarrow\sigmabar(d_{i,1})
\end{aligned} \label{property: Sv1} \tag{Sv1}
\end{align*}
\end{minipage}
\hfill
\begin{minipage}{0.41\textwidth}
\begin{align*}
\begin{aligned}
\indbit_1^{\sigma}=0\Rightarrow\sigma(e_{*,*,*})=b_2 \\
\indbit_1^{\sigma}=1\Rightarrow\sigma(e_{*,*,*})=g_1
\end{aligned}\label{property: Esc1} \tag{Esc1}\\
\sigma(e_{*,*,*})=g_1 \label{property: Esc2} \tag{Esc2}\\
\sigmabar(eg_{i,j})\wedge\neg\sigmabar(eb_{i,j}) \label{property: Esc3} \tag{Esc3}\\
\sigmabar(eb_{i,j})\wedge\neg\sigmabar(eg_{i,j}) \label{property: Esc4} \tag{Esc4}\\
\sigmabar(eg_{i,j})\wedge\sigmabar(eb_{i,j}) \label{property: Esc5} \tag{Esc5}\\
\sigmabar(b_i)=\sigmabar(d_{i,\indbit_{i+1}}^{\sigma}) \label{property: Bac1} \tag{Bac1}\\
\sigmabar(b_i)\Rightarrow \sigmabar(g_i)=\indbit_{i+1}^{\sigma} \label{property: Bac2} \tag{Bac2}\\
\sigmabar(b_i)\Rightarrow\nsigmabar(d_{i,1-\indbit_{i+1}^{\sigma}}) \label{property: Bac3} \tag{Bac3} 
\end{align*}
\end{minipage}
}

\bigskip

Before giving the definition of the phases, we introduce additional properties.
These properties are not used for the definition of the phases and are related to the occurrence records of cycle edges.
These properties in particular yield insights regarding the parameter $t_{\bit}$ used in \Cref{table: Occurrence Records}.
The occurrence records of cycle edges are rather complicated, hence these additional properties that help us in proving that \Cref{table: Occurrence Records} describes their occurrence records correctly.
They are furthermore part of the canonical conditions, a set of properties every canonical strategy has.

{\footnotesize
\allowdisplaybreaks
\begin{align*}
\sigma(d_{i,j,k})=F_{i,j}\wedge(\bit_i=0\vee\bit_{i+1}\neq j)\implies \occrec^{\sigma}(d_{i,j,k},F_{i,j})<\floor{\frac{\bit+1}{2}} \label{property: Or1} \tag{Or1}\\
\indbit^{\sigma}_{i}=0\vee\indbit^{\sigma}_{i+1}\neq j\implies [\occrec^{\sigma}(d_{i,j,k},F_{i,j})=\ell^{\bit}(i,j,k)+1\Leftrightarrow\sigma(d_{i,j,k})=F_{i,j}] \label{property: Or2} \tag{Or2}\\
\begin{aligned} 
			\occrec^{\sigma}(d_{i,j,k},F_{i,j})&=\ell^{\bit}(i,j,k)-1\wedge\occrec^{\sigma}(d_{i,j,k},F_{i,j})\neq\floor{\frac{\bit+1-k}{2}}\\
				&\Longleftrightarrow \bit\text{ is odd}, \nexists l\in\mathbb{N}\colon\bit+1=2^l, i=\nsb(\bit+1), j\neq\bit_{i+1}, k=0.
\end{aligned} \label{property: Or3} \tag{Or3}\\
\sigma(d_{i,j,k})\neq F_{i,j}\implies\occrec^{\sigma}(d_{i,j,k},F_{i,j})\in\left\{\floor{\frac{\bit+1}{2}}-1,\floor{\frac{\bit+1}{2}}\right\} \label{property: Or4} \tag{Or4}
\end{align*}
}

\Cref{table: Definition of Phases} is used to define the five phases, see \Cref{definition: Phase k Strategy}.
It contains one column listing all properties and one column per phase.
A strategy is called a Phase-$k$-strategy if it has the properties listed in the corresponding column (resp. if it has the property for the respective indices if the property depends on one or two indices).
A '-' signifies that it is not specified whether the strategy has the corresponding property.
It thus may or may not have it.
%Also note that we introduce the term ``real Phase-3-strategy'' which is a Phase-3-strategy that additionally has \Cref{property: Cc2}.

{\footnotesize
\begin{longtable}[ht]{|c||c|c|c|c|c|}
\hline%
\endfirsthead
Property						&Phase 1	&Phase 2				&Phase 3												&Phase 4										&Phase 5 \\\hline\hline
(\ref{property: Bac1})$_{i}$	&$i\in[n]$	&$i>\relbit{\sigma}$	&$i>1$													&$i\in[n]$										&$i\in[n]$\\
(\ref{property: Bac2})$_{i}$	&$i\in[n]$	&$i\geq\relbit{\sigma}$	&$i>1$													&$i\in[n]$										&$i\in[n]$\\	
%(\ref{property: Bac3})$_{i}$	&$i\in[n]$	&$i\in[n]$				&$i\in[n]$												&$i>1$											&$i>1$\\
(\ref{property: Bac3})$_{i}$	&$i\in[n],i\neq\nsb$	&$i>\relbit{\sigma}$	&$i>1,i\neq\relbit{\sigma}$								&$i\in[n]$										&$i\in[n]$\\				
(\ref{property: Usv1})$_{i}$	&$i\in[n]$	&$i\geq\relbit{\sigma}$	&$i\geq\relbit{\sigma}$									&$i\geq\nsb$									&$i\in[n]$\\
(\ref{property: Usv2})$_{i,j}$	&-			&$(i,1-\indbit^{\sigma}_{i+1})\colon i<\relbit{\sigma}$				&$(i,*)\colon i<\relbit{\sigma}$	&$(i,\indbit_{i+1}^{\sigma})\colon i<\nsb$		&-\\
(\ref{property: Esc1})			&True		&-						&-														&-												&False*\\
(\ref{property: Esc2})			&-			&True					&-														&-												&-\\
%(\ref{property: Esc3})			&-			&-						&-														&-												&- \\
(\ref{property: Esc4})$_{i,j}$	&-			&-						&-														&$S_1$											&- \\
(\ref{property: Esc5})$_{i,j}$	&-			&-						&-														&$S_2$											&-\\
(\ref{property: Rel1})			&True		&-						&-														&True											&True\\
(\ref{property: Rel2})			&-			&True					&True													&False											&False\\
(\ref{property: Cc1})$_{i}$		&$i\in[n]$	&$i\in[n]$				&$i\in[n]$												&$i\in[n]$										&$i\in[n]$ \\			
(\ref{property: Cc2})			&-			&-						&-														&True											&True\\
(\ref{property: Sv1})$_{i}$		&$i\in[n]$	&$i\in[n]$				&-														&-												&-*\\
$\indbit^{\sigma}=$				&$\bit$		&$\bit+1$				&$\bit+1$												&$\bit+1$										&$\bit+1$\\\hline										
Special	&Phase 2: 	&\multicolumn{4}{l|}{$\exists i<\relbit{\sigma}\colon$(\ref{property: Usv3})$_{i}\wedge\neg$(\ref{property: Bac2})$_{i}\wedge\neg$(\ref{property: Bac3})$_{i}$}\\
		&Phase 3:	&\multicolumn{4}{l|}{A Phase 3 strategy that has \Cref{property: Cc2} is called \emph{proper} Phase-3-strategy} \\		
		&Phase 4: 	&\multicolumn{4}{l|}{$\exists i<\nsb(\bit+1)\colon$(\ref{property: Usv2})$_{i,1-\indbit_{i+1}^{\sigma}}$}\\
		&Phase 5:	&\multicolumn{4}{l|}{*If a strategy has \Cref{property: Esc1} and there is an index $i$ such that}\\
		&			&\multicolumn{4}{l|}{it does not have \Cref{property: Sv1}$_{i}$, it is defined as a Phase-5-strategy}\\
\hline
\caption{Definition of the phases.
	The entries show for which set of indices the strategy has the corresponding property resp. whether the strategy has the property at all.
	%A '-' signifies that it is not specified whether the strategy has the corresponding property.
	The last row contains assumptions and further properties used for the definition of the phases.
	We define $[n]=\{1,\dots,n\}$ and $\nsb\coloneqq\nsb(\bit+1)$.} \label{table: Definition of Phases}
\end{longtable}
}

\Cref{table: Further strategy assumptions} contains sets of pairs of indices $(i,j)$ that are used for defining the phases or within several later proofs and statements.

\vspace*{-2pt}

{\footnotesize
\begin{longtable}{|c|l|}\hline
$S_1=$ 	&$\{(i,1-\indbit^{\sigma}_{i+1})\colon i\leq \nsb)-1\}\cup$\\
		&$\{(i,1-\indbit^{\sigma}_{i+1})\colon i\in\{\nsb,\dots,m-1\}\wedge\indbit^{\sigma}_i=0\}\cup $\\
		&$\begin{cases}\emptyset &\exists k\in\mathbb{N}\colon \bit+1=2^k\\\{(\nsb,1-\indbit^{\sigma}_{\nsb+1})\}, &\nexists k\in\mathbb{N}\colon \bit+1=2^k \end{cases} $\\\hline
$S_2=$	&$\{(i,\indbit^{\sigma}_{i+1})\colon i\leq \nsb(\bit+1)-1\}\cup$\\
		&$\{(i,1-\indbit^{\sigma}_{i+1})\colon i\in\{\nsb(\bit+1)+1,\dots,m\}\wedge\indbit^{\sigma}_i=1\}\cup $\\
		&$\{(i,\indbit^{\sigma}_{i+1})\colon i\in\{\nsb(\bit+1),\dots,m-1\}\wedge\indbit^{\sigma}_i=0\}\cup $\\
		&$\{(i,k)\colon i>m, k\in\{0,1\}\}\cup$\\
		&$\begin{cases}\{(\nsb(\bit+1), 1)\} &\exists k\in\mathbb{N}\colon \bit+1=2^k\\\emptyset, &\nexists k\in\mathbb{N}\colon \bit+1=2^k \end{cases} $\\\hline
%$X_k$= 	&$\begin{cases} \emptyset, &\exists l\colon \indbit^{\sigma}=2^l \\\{(d_{\nsb,1-\indbit^{\sigma}_{\nsb+1},k},F_{\nsb,1-\indbit^{\sigma}_{\nsb+1}})\}\cup\bigcup\limits_{\substack{i=\nsb+1\\\indbit^{\sigma}_i=0}}^{m-1}\{(d_{i,1-\indbit^{\sigma}_{i+1},k},F_{i,1-\indbit^{\sigma}_{i+1}})\}&\text{otherwise}\end{cases}$\\\hline
%		&			&\multicolumn{4}{l|}{\emph{True} Phase 3 strategy $\Longleftrightarrow$ fulfills \Cref{property: Cc2}}\\\hline
$S_3=$	&$\{(i,1-\indbit^{\sigma}_{i+1})\colon i\in\{1,\dots,u\}\}\cup$\\
		&$\{(i,1-\indbit^{\sigma}_{i+1})\colon i\in\{u+1,\dots,m\}\wedge\indbit^{\sigma}_{i}=1\}\cup$\\
		&$\{(i,\indbit^{\sigma}_{i+1})\colon i\in\{u+1,\dots,m-1\}\wedge\indbit^{\sigma}_i=0\}\cup$\\
		&$\{(i,k)\colon i>m, k\in\{0,1\}\}\cup\{(u,\indbit^{\sigma}_{u+1})\}$\\\hline
$S_4=$	&$\{(i,1-\indbit^{\sigma}_{i+1})\colon i\in\{u+1,\dots,m-1\}\wedge\indbit^{\sigma}_{i}=0\}$\\\hline
\caption{Sets used for the definition of the phases.
We use the abbreviations $m=\max\{i\colon\indbit^\sigma_i=1\}$ and $u=\min\{i\colon\indbit^\sigma_i=0\}$ as well as $\nsb=\nsb(\bit+1)$.} \label{table: Further strategy assumptions}
\end{longtable}
}

The next table gives an overview over the strategies at the beginning of each phase.
More precisely, it contains properties that the strategies at the beginning of the different phases have.
It also gives an overview over the different combinations of phases, contexts and parameters $\nsb$ that can and cannot occur.
We also introduce the following notation.
For strategies $\sigma,\sigma'$ with $\sigma\in\reach{\sigma'}$, the sequence of improving switches that the Strategy Improvement Algorithm applies when starting with $\sigma$ until it reaches $\sigma'$ is denoted by $\applied{\sigma}{\sigma'}$.

{
\footnotesize
\begin{longtable}{|c||C{4.5cm}|C{7cm}|C{1.5cm}|}\hline
\multirow{2}{*}{Phase}		&\multirow{2}{*}{$\nsb=1$}	&\multicolumn{2}{c|}{$\nsb>1$}\\\cdashline{3-4}
							&							&PG			&MDP			\\\hline\hline
1							&\multicolumn{3}{c|}{Canonical strategy for $\bit$ fulfilling the canonical conditions}\\\hline
\multirow{5}{*}{2}			&\multirow{5}{*}{-}			&\multicolumn{2}{c|}{$\sigma(d_{i,j,k})\neq F_{i,j}\Rightarrow\occrec^{\sigma}(d_{i,j,k},F_{i,j})=\floor{\frac{\bit+1}{2}}$}\\
							&							&\multicolumn{2}{c|}{$(g_i,F_{i,j})\in\applied{\canstrat}{\sigma}\Rightarrow[\bit_i=0\wedge\bit_{i+1}\neq j]\vee i=\nsb$ and $F_{i,j}$ is closed}\\
							&							&\multicolumn{2}{c|}{$\applied{\canstrat}{\sigma}\subseteq\D^1\cup\G$}\\
							&							&\multicolumn{2}{c|}{$\sigma(g_{\nsb})=F_{\nsb,\indbit_{\nsb+1}^{\sigma}}$ and $\sigma(g_i)=F_{i,1-\indbit^{\sigma}_{i+1}}$ for all $i<\nsb$}\\
							&							&\multicolumn{2}{c|}{$i<\nsb\Rightarrow \sigmabar(d_{i})$ and \Cref{property: Usv3}$_i$}\\\hline
\multirow{3}{*}{3}			&\multicolumn{3}{c|}{$\sigma(d_{i,j,k})\neq F_{i,j}\Rightarrow\occrec^{\sigma}(d_{i,j,k},F_{i,j})=\occrec^{\canstrat}(d_{i,j,k},F_{i,j})=\floor{\frac{\bit+1}{2}}$}\\
							&\multicolumn{3}{c|}{$\sigma(s_{i,*})=h_{i,*}, \sigma(g_i)=F_{i,1-\indbit^{\sigma}_{i+1}}$ and $\sigmabar(d_i)$ for all $i<\nsb$ as well as $\sigma(g_{\nsb})=F_{\nsb,\bit_{\nsb+1}}$}\\
							&\multicolumn{3}{c|}{$\applied{\canstrat}{\sigma^3}\subseteq\D^1\cup\G\cup\S\cup\B$ and $(g_i,F_{i,j})\in\applied{\canstrat}{\sigma}\Rightarrow[\bit_i=0\wedge\bit_{i+1}\neq j]\vee i=\nsb$ and $F_{i,j}$ is closed}\\\hline
\multirow{8}{*}{4}			&\multirow{9}{*}{-}	&$\relbit{\sigma}=\min\{i\colon\indbit^{\sigma}_i=0\}$																	&\multirow{8}{*}{-}\\
							&					&$\sigma(d_{i,j,k})=F_{i,j}\Leftrightarrow\indbit^{\sigma}_{i}=1\wedge(\bit+1)_{i+1}=j$													&\\
							&					&$(i,j)\in S_1\Rightarrow\sigmabar(eb_{i,j})\wedge\nsigmabar(eg_{i,j})$																			&\\
							&					&$(i,j)\in S_2\Rightarrow\sigmabar(eb_{i,j})\wedge\sigmabar(eg_{i,j})$																			&\\
							&					&$(g_i,F_{i,j})\in\applied{\canstrat}{\sigma}\Rightarrow[\bit_i=0\wedge\bit_{i+1}\neq j]\vee i=\nsb$									&\\
							&					&$(g_i,F_{i,j})\in\applied{\canstrat}{\sigma}\Rightarrow$ $F_{i,j}$ is closed															&\\	
							&					&$\sigma(e_{i,j,k})=b_2\Rightarrow\occrec^{\sigma}(d_{i,j,k},F_{i,j})=\occrec^{\canstrat}(d_{i,j,k},F_{i,j})$	&\\
							&					&$\sigma(e_{i,j,k})=b_2\Rightarrow\occrec^{\sigma}(d_{i,j,k},F_{i,j})=\floor{\frac{\bit+1}{2}}$	&\\\hline
\multirow{7}{*}{5}			&\multicolumn{3}{c|}{$\relbit{\sigma}=\min\{i\colon\indbit^{\sigma}_{i+1}=0\}$}		\\
							&\multicolumn{3}{c|}{$\sigma(d_{i,j,k})=F_{i,j}\Leftrightarrow\indbit^{\sigma}_{i}=1\wedge(\bit+1)_{i+1}=j$}		\\
							&\multicolumn{3}{c|}{$(g_i,F_{i,j})\in\applied{\canstrat}{\sigma}\Rightarrow[\bit_i=0\wedge\bit_{i+1}\neq j]\vee i=\nsb$}		\\
							&\multicolumn{3}{c|}{$\sigma(e_{i,j,k})=t^{\rightarrow}\Rightarrow\occrec^{\sigma}(d_{i,j,k},F_{i,j})=\occrec^{\canstrat}(d_{i,j,k},F_{i,j})=\floor{\frac{\bit+1}{2}}$}\\\cdashline{2-4}
							&$(i,j)\in S_4\Rightarrow\sigmabar(eg_{i,j})\wedge\nsigmabar(eb_{i,j})$	&\multicolumn{2}{c|}{$(i,j)\in S_1\Rightarrow\sigmabar(eb_{i,j})\wedge\nsigmabar(eg_{i,j})$}\\
							&$(i,j)\in S_3\Rightarrow\sigmabar(eg_{i,j})\wedge\sigmabar(eb_{i,j})$		&\multicolumn{2}{c|}{$(i,j)\in S_2\Rightarrow\sigmabar(eb_{i,j})\wedge\sigmabar(eg_{i,j})$}\\
							&																							&\multicolumn{2}{c|}{$i<\nsb\Rightarrow\sigmabar(g_i)=1-\indbit^{\sigma}_{i+1}$}\\\hline
1							&\multicolumn{3}{c|}{Canonical strategy for $\bit+1$ fulfilling the canonical conditions}\\\hline
\caption{Properties that specific Phase-$k$-strategies have.
To simplify notation, we define $t^{\rightarrow}\coloneqq g_1$ if $\nsb=1$ and $t^{\rightarrow}\coloneqq b_2$ if $\nsb>1$.
A '-' signifies that the corresponding combination of phase, context and $\nsb$ does not occur during the execution of the algorithm.
We do not interpret the header as the first row of this table.} \label{table: Properties Of Phase k Strategies}
\end{longtable}
}

The next table gives an overview over the set of improving switches at the beginning of the different phases.
It thus in particular describes the same strategies whose properties are summarized in \ref{table: Properties Of Phase k Strategies}.
It also shows which phases can actually occur depending on whether we consider PG or MDP context and depending on the least significant set bit of the next number.

{

\footnotesize
\begin{longtable}[ht]{|c|C{5.5cm}|C{7cm}|c|}
\hline%
\endfirsthead

\multirow{2}{*}{Phase}		&\multirow{2}{*}{$\nsb=1$}	&\multicolumn{2}{c|}{$\nsb>1$}	\\\cdashline{3-4}
							&							&PG			&MDP				\\\hline	
1							&\multicolumn{3}{c|}{$\mathfrak{D}^{\sigma}\coloneqq\{(d_{i,j,k},F_{i,j})\colon\sigma(d_{i,j,k})\neq F_{i,j}\}$} \\\hline
2							&-								&\multicolumn{2}{c|}{$\mathfrak{D}^{\sigma}\cup\{(b_{\nsb},g_{\nsb}), (s_{\nsb-1,1},h_{\nsb-1,1})\}$}\\\hline
3							&$\mathfrak{D}^{\sigma}\cup\{(b_1,g_1)\}\cup\{(e_{*,*,*},g_1)\}$	&\multicolumn{2}{c|}{$\mathfrak{D}^{\sigma}\cup\{(b_1,b_2)\}\cup\{(e_{*,*,*},b_2)\}$}\\\hline
4							&-							& $\mathfrak{E}^{\sigma}\cup \{(s_{\nsb-1,0},b_1)\}\cup\{(s_{i,1},b_1)\colon i\leq\nsb-2\} \cup X_0\cup X_1$					&-\\\hline
5							&$\displaystyle\mathfrak{E}^{\sigma}\cup \bigcup^{m-1}_{\substack{i=\relbit{\sigma}+1\\\indbit^{\sigma}_i=0}}\{(d_{i,1-\indbit^{\sigma}_{i+1},*},F_{i,1-\indbit^{\sigma}_{i+1}})\}$	&\multicolumn{2}{C{8cm}|}{$\displaystyle\mathfrak{E}^{\sigma} \cup \bigcup^{\nsb-1}_{i=1}\{d_{i,1-\indbit^{\sigma}_{i+1},*}, F_{i,-1-\indbit^{\sigma}_{i+1}})\}\cup X_0\cup X_1$}\\\hline
1							&\multicolumn{3}{c|}{$\mathfrak{D}^{\sigma}$}\\\hline\hline
\multicolumn{4}{|c|}{$		\displaystyle X_k\coloneqq\begin{cases}
			\emptyset, &\bit+1\text{ is a power of two}\\
			\{(d_{\nsb,1-\indbit^{\sigma}_{\nsb},k},F_{\nsb,1-\indbit^{\sigma}_{\nsb}})\}\cup\bigcup\limits_{\substack{i=\nsb+1\\\indbit_{i}=0}}^{m-1}\{(d_{i,1-\indbit^{\sigma}_{i+1},k},F_{i,1-\indbit^{\sigma}_{i+1}})\}, &\text{otherwise}\end{cases}.
$}\\\hline
\caption{Improving switches at the beginning of different phases when starting with a canonical strategy $\canstrat$ for $\bit$.
We use $\nsb\coloneqq\nsb(\bit+1)$ and $m\coloneqq\max\{i\colon\sigma(b_i)=g_i\}$ to simplify the notation.
We further define $\mathfrak{E}^{\sigma}\coloneqq\{(d_{i,j,k},F_{i,j}),(e_{i,j,k},b_2)\colon\sigma(e_{i,j,k})=g_1\}$ if $\nsb>1$ and, analogously, $\mathfrak{E}^{\sigma}\coloneqq\{(d_{i,j,k},F_{i,j}),(e_{i,j,k},g_1)\colon\sigma(e_{i,j,k})=b_2\}$ if $\nsb=1$.
Note that we do not interpret $1$ as a power of two.} \label{table: Phases}
\end{longtable}
}
